# Supplementary material for: TMO: Textured Mesh Acquisition of Objects with a Mobile Device by using Differentiable Rendering
Source: arXiv:2303.15060 source file (2023-03-27)
Supplement: Supplementary file 1 [file supplmentary.tex]

% CVPR 2023 Paper Template
% based on the CVPR template provided by Ming-Ming Cheng (https://github.com/MCG-NKU/CVPR_Template)
% modified and extended by Stefan Roth (stefan.roth@NOSPAMtu-darmstadt.de)

\documentclass[10pt,onecolumn,letterpaper]{article}

%%%%%%%%% PAPER TYPE  - PLEASE UPDATE FOR FINAL VERSION
% \usepackage[review]{cvpr}      % To produce the REVIEW version
\usepackage{cvpr}              % To produce the CAMERA-READY version
%\usepackage[pagenumbers]{cvpr} % To force page numbers, e.g. for an arXiv version

% Include other packages here, before hyperref.
\usepackage{graphicx}
\usepackage{amsmath}
\usepackage{amssymb}
\usepackage{booktabs}
% 임의로 추가한 package
\usepackage{multirow}
\usepackage{booktabs}
\usepackage{caption}

% Algorithm package
\usepackage{algorithm}
\usepackage{algorithmic}
\usepackage{algpseudocode}

% It is strongly recommended to use hyperref, especially for the review version.
% hyperref with option pagebackref eases the reviewers' job.
% Please disable hyperref *only* if you encounter grave issues, e.g. with the
% file validation for the camera-ready version.
%
% If you comment hyperref and then uncomment it, you should delete
% ReviewTempalte.aux before re-running LaTeX.
% (Or just hit 'q' on the first LaTeX run, let it finish, and you
%  should be clear).
\usepackage[pagebackref,breaklinks,colorlinks]{hyperref}

% Support for easy cross-referencing
\usepackage[capitalize]{cleveref}
\crefname{section}{Sec.}{Secs.}
\Crefname{section}{Section}{Sections}
\Crefname{table}{Table}{Tables}
\crefname{table}{Tab.}{Tabs.}

%%%%%%%%% PAPER ID  - PLEASE UPDATE
 % *** Enter the CVPR Paper ID here

\begin{document}

%%%%%%%%% TITLE - PLEASE UPDATE
\title{TMO: Textured Mesh Acquisition of Objects with a Mobile Device by using Differentiable Rendering 

Supplementary Material}

% \author{First Author\\
% Institution1\\
% Institution1 address\\
% {\tt\small firstauthor@i1.org}
% % For a paper whose authors are all at the same institution,
% % omit the following lines up until the closing ``}''.
% % Additional authors and addresses can be added with ``\and'',
% % just like the second author.
% % To save space, use either the email address or home page, not both
% \and
% Second Author\\
% Institution2\\
% First line of institution2 address\\
% {\tt\small secondauthor@i2.org}
% }
\author{Jaehoon Choi\:\textsuperscript{\rm 1,2} \:\: Dongki Jung\:\textsuperscript{\rm 1} \:\: Taejae Lee\:\textsuperscript{\rm 1} \:\: Sangwook Kim\:\textsuperscript{\rm 1} \:\: Youngdong Jung\:\textsuperscript{\rm 1} \\ Dinesh Manocha\:\textsuperscript{\rm 2} \:\:Donghwan Lee\:\textsuperscript{\rm 1}\\
$^{1}$NAVER LABS \:\: $^{2}$University of Maryland}

\maketitle

%%%%%%%%% BODY TEXT
% mesh depth map
% implementation Detail 설명
% monosdf 결과 
% hyperparameter 수치
\section{Data Collection}
We provide specific properties of our data collection process. As mentioned in the manuscript, ARKit-video collects long video sequences to apply the RGBD SLAM methods \cite{dai2017bundlefusion} to extract poses and fuse a 3D model. 
However, we fail to apply the state-of-the-art RGBD SLAM algorithm \cite{dai2017bundlefusion} for accurate pose estimation due to noisy depth measurements. Instead, we utilize accurate poses from our RGBD-aided Structure from Motion (SfM) for geometry reconstruction and texture optimization. ARKit-video includes \textit{recliner chair}, \textit{cafe stand}, \textit{delivery robot}, \textit{office chair}, and \textit{camera stand}. We can apply TSDF-fusion \cite{izadi2011kinectfusion} with poses from RGBD-adied SfM to reconstruct geometry in Fig. 6. in the manuscript because of the video sequence.   
AR-capture includes \textit{robot arm 1}, \textit{robot arm 2}, \textit{plant}, \textit{tree}, \textit{sofa}, \textit{bike}, \textit{recliner chair}, \textit{cafe stand}, \textit{delivery robot}, \textit{office chair}, and \textit{camera stand}. 
Except for \textit{sofa} and \textit{tree}, AR-capture contains less than fifty images. The \textit{sofa} contains 108 images because the mobilephone camera has difficulty capturing this sofa due to the large size (This sofa can seat up to 15 people). We require a number of images to capture the whole shape of \textit{sofa}. The \textit{tree} contains 111 images and is also large size object. In addition to this, the \textit{tree} has a very complex shape (e.g. leaf) and thin structure (e.g. stem).

\section{Implementation Details}
In preprocessing stage, we apply both single-view and multi-view filtering two times. We regard 10 neighboring frames as source images and set the threshold $\epsilon$ to 0.1. We keep depth pixels if the ratio of inliers is greater than 80\%. We remove depth points larger than 2.55m. 
Our RGBD-aided Structure from Motion (SfM) is based on COLMAP \cite{schonberger2016structure} implemented in C++. Similar to the existing COLMAP, we use Ceres Solver to perform bundle adjustment.    
After SfM, we apply MVS algorithm \cite{xu2020planar,schonberger2016pixelwise} to provide the depth and normal for geometry reconstruction. Here, we also leverage the filtering algorithm to remove the noisy values for the depth and normal maps obtained from the MVS algorithm. For the first stage of trainning process in Sec. 3.2, we set $w_{d}$ to 1e-5 and $w_{n}$ to 1e-3. After the first stage, we build sparse voxel volume around surfaces obtained from mesh. We set a depth level of octree to 8 for all classes. During the training for two MLPs (the SDF network and color network), we also model the background by NeRF++ \cite{zhang2020nerf++}. The sampling strategy is also similar to the NeuS \cite{wang2021neus}.       
For geometry reconstruction and texture optimization, we use 41 - 108 images at 1280\:x\:720 pixels sampled from video sequence of ARKit-video. Since AR-capture has large images at 4032x3096 resolutions, we resize their resolution to 1008x774 resolution for geometry reconstruction and texture optimization. The LiDAR sensor in the iOS device provides depth maps and confidence maps with size 256\:x\:192. For mesh simplification, we exploit the quadric mesh simplification algorithm provided by \cite{open3d}. The learning rates for texture optimization start from 1e-3 and decay the learning rate by 0.1 once the epoch reaches 500 and 2000 respectively. As mentioned in manuscript, we use the public github code for the classical MVS \cite{xu2020planar,schonberger2016pixelwise} and texture mapping \cite{waechter2014TexRecon} which are implemented in C++. We implement all geometry reconstruction and texture optimization in PyTorch \cite{paszke2017automatic} and conduct all experiments on V100 GPU.

% How many images?
% AR_capture: robot arm1 : 35,42,41, 39,  / sofa 146, plant2 111
% AR_video: 70 , 41, 108, 79, 68
% classical MVS
% NeuS 
% Decimation 
% MVS texturing
% Texture adjoin 

\section{Additional Qualitative Comparisons}
In the manuscript, we only show the reconstructed texture of \textit{delivery robot}, \textit{recliner chair}, \textit{robot arm 1}, and \textit{office chair} (refer the Fig.\:7 in the manuscript) due to the limited space. Here, we visualize our results of other objects: \textit{cafe stand}, \textit{sofa}, \textit{plant}, \textit{bike}, \textit{robot arm2}, \textit{tree}, and \textit{camera stand}. We compare our method with four different methods following the manuscript. 
Compared to these methods, our visual results are visually sharper and perceptually closer to the original scene. Furthermore, we apply our method to 3D indoor scene and show the feasibility of reconstructing the textured mesh for 3D indoor scenes.       

\begin{figure}[h]
  \centering
    \vspace{-8mm}
    \includegraphics[width=0.9\linewidth,keepaspectratio]{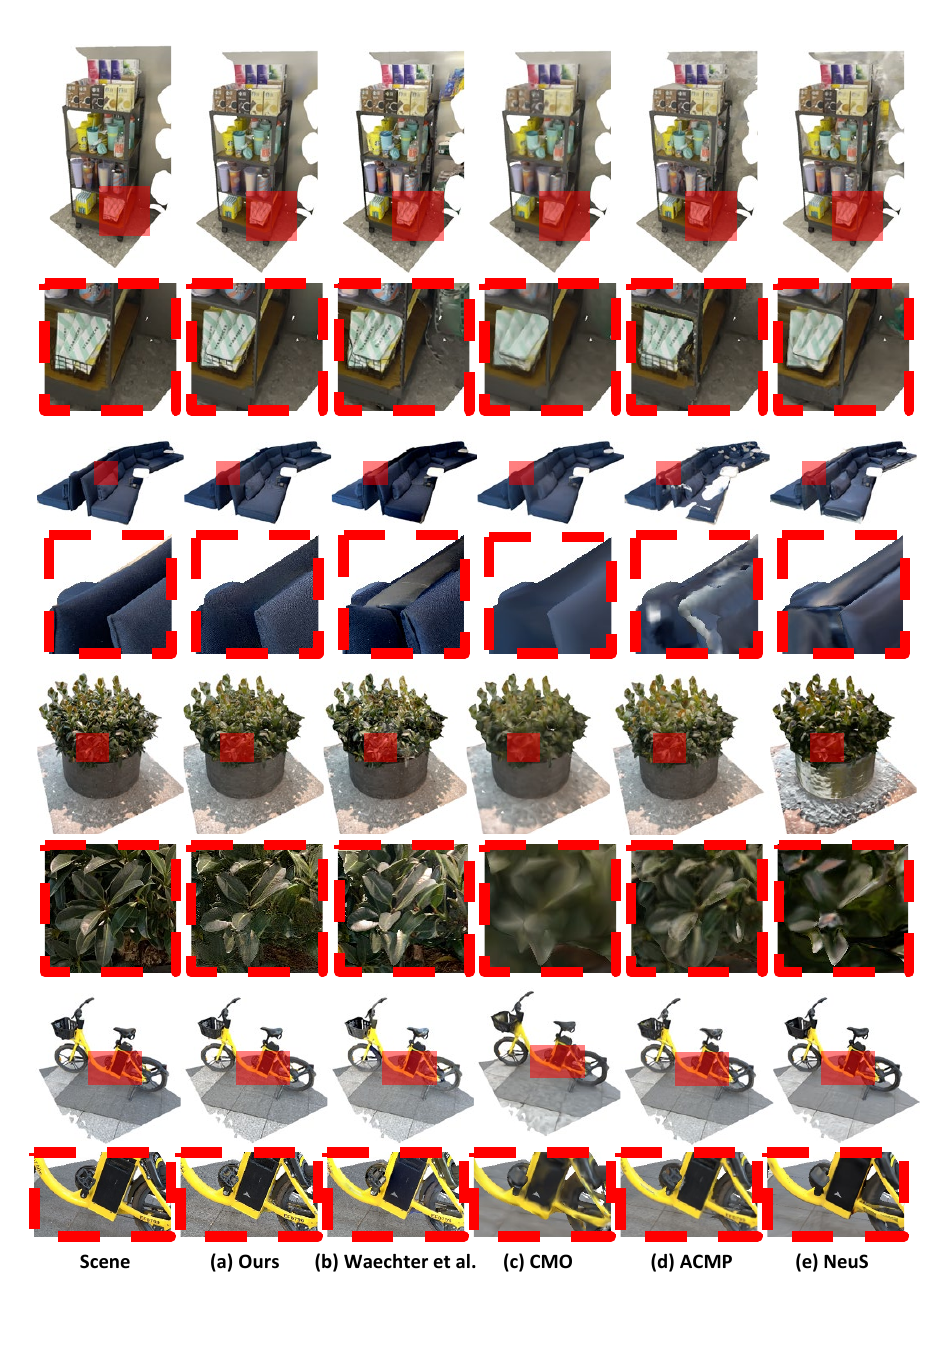}
    \vspace{-15mm}
   \caption{Qualitative comparison between (a) Ours,  (b) Waechter et al. \cite{waechter2014TexRecon}, (c) CMO \cite{zhou2014colormapoptimization}, (d) ACMP \cite{xu2020planar}, and (e) NeuS \cite{wang2021neus}. From top to bottom, we show the results of \textit{cafe stand}, \textit{sofa}, \textit{plant}, and \textit{bike}. We collect \textit{bike} at the outdoor environment in uncontrolled settings. The \textit{sofa} has the large size (it can seat up to 15 people). Our method can perform 3D reconstruction and texture mapping for the large object and the object under the outdoor environment.}
   \vspace{-15mm}
   \label{fig:onecol}
\end{figure}

\newpage

\begin{figure}[h]
  \centering
    \includegraphics[width=0.8\linewidth,keepaspectratio]{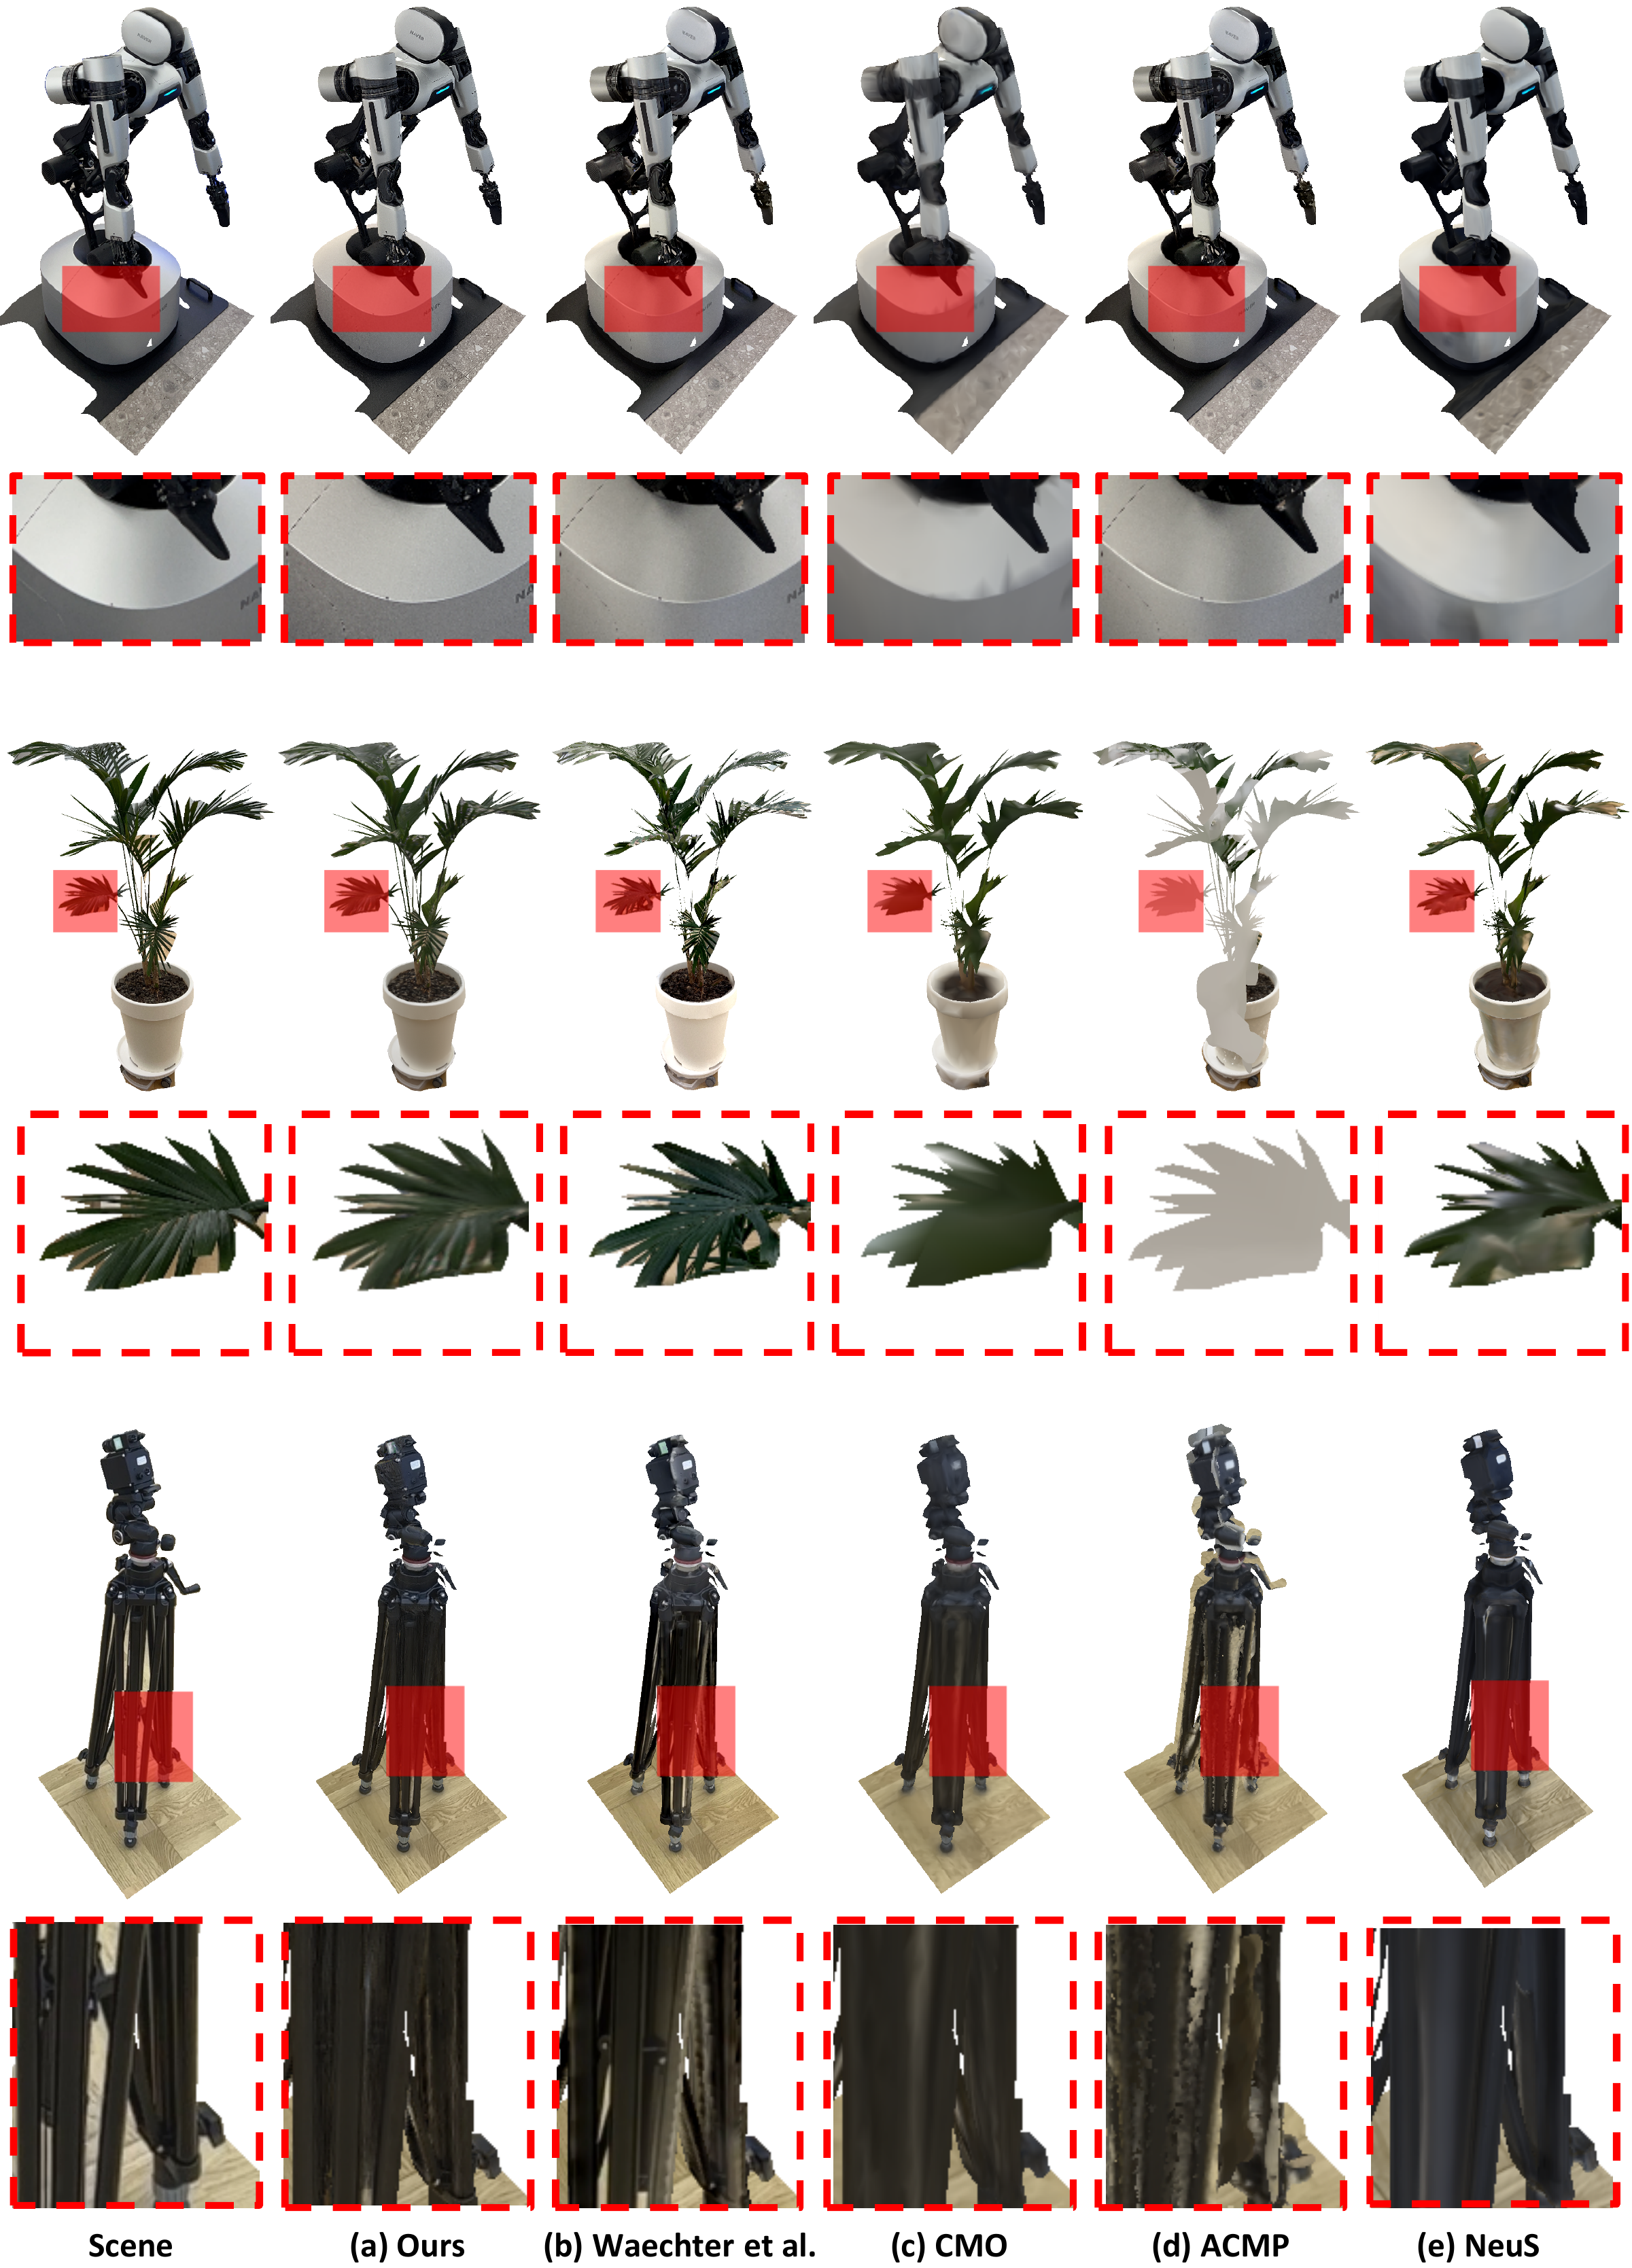}
    % \vspace{-3mm}
   \caption{Qualitative comparison between (a) Ours,  (b) Waechter et al. \cite{waechter2014TexRecon}, (c) CMO \cite{zhou2014colormapoptimization}, (d) ACMP \cite{xu2020planar}, and (e) NeuS \cite{wang2021neus}. From top to bottom, we show the results of \textit{robot arm2}, \textit{tree}, and \textit{camera stand}.  The \textit{tree} has a very complex shape (e.g. leaf) and thin structure (e.g. stem). Also, the \textit{camera stand} has a thin structure. Our method can perform 3D reconstruction and texture mapping for objects with complex shapes and thin structures.             
   }
   % \vspace{-4mm}
   \label{fig:onecol}
\end{figure}

\newpage

\begin{figure}[t]
  \centering
    \includegraphics[width=\textwidth,keepaspectratio]{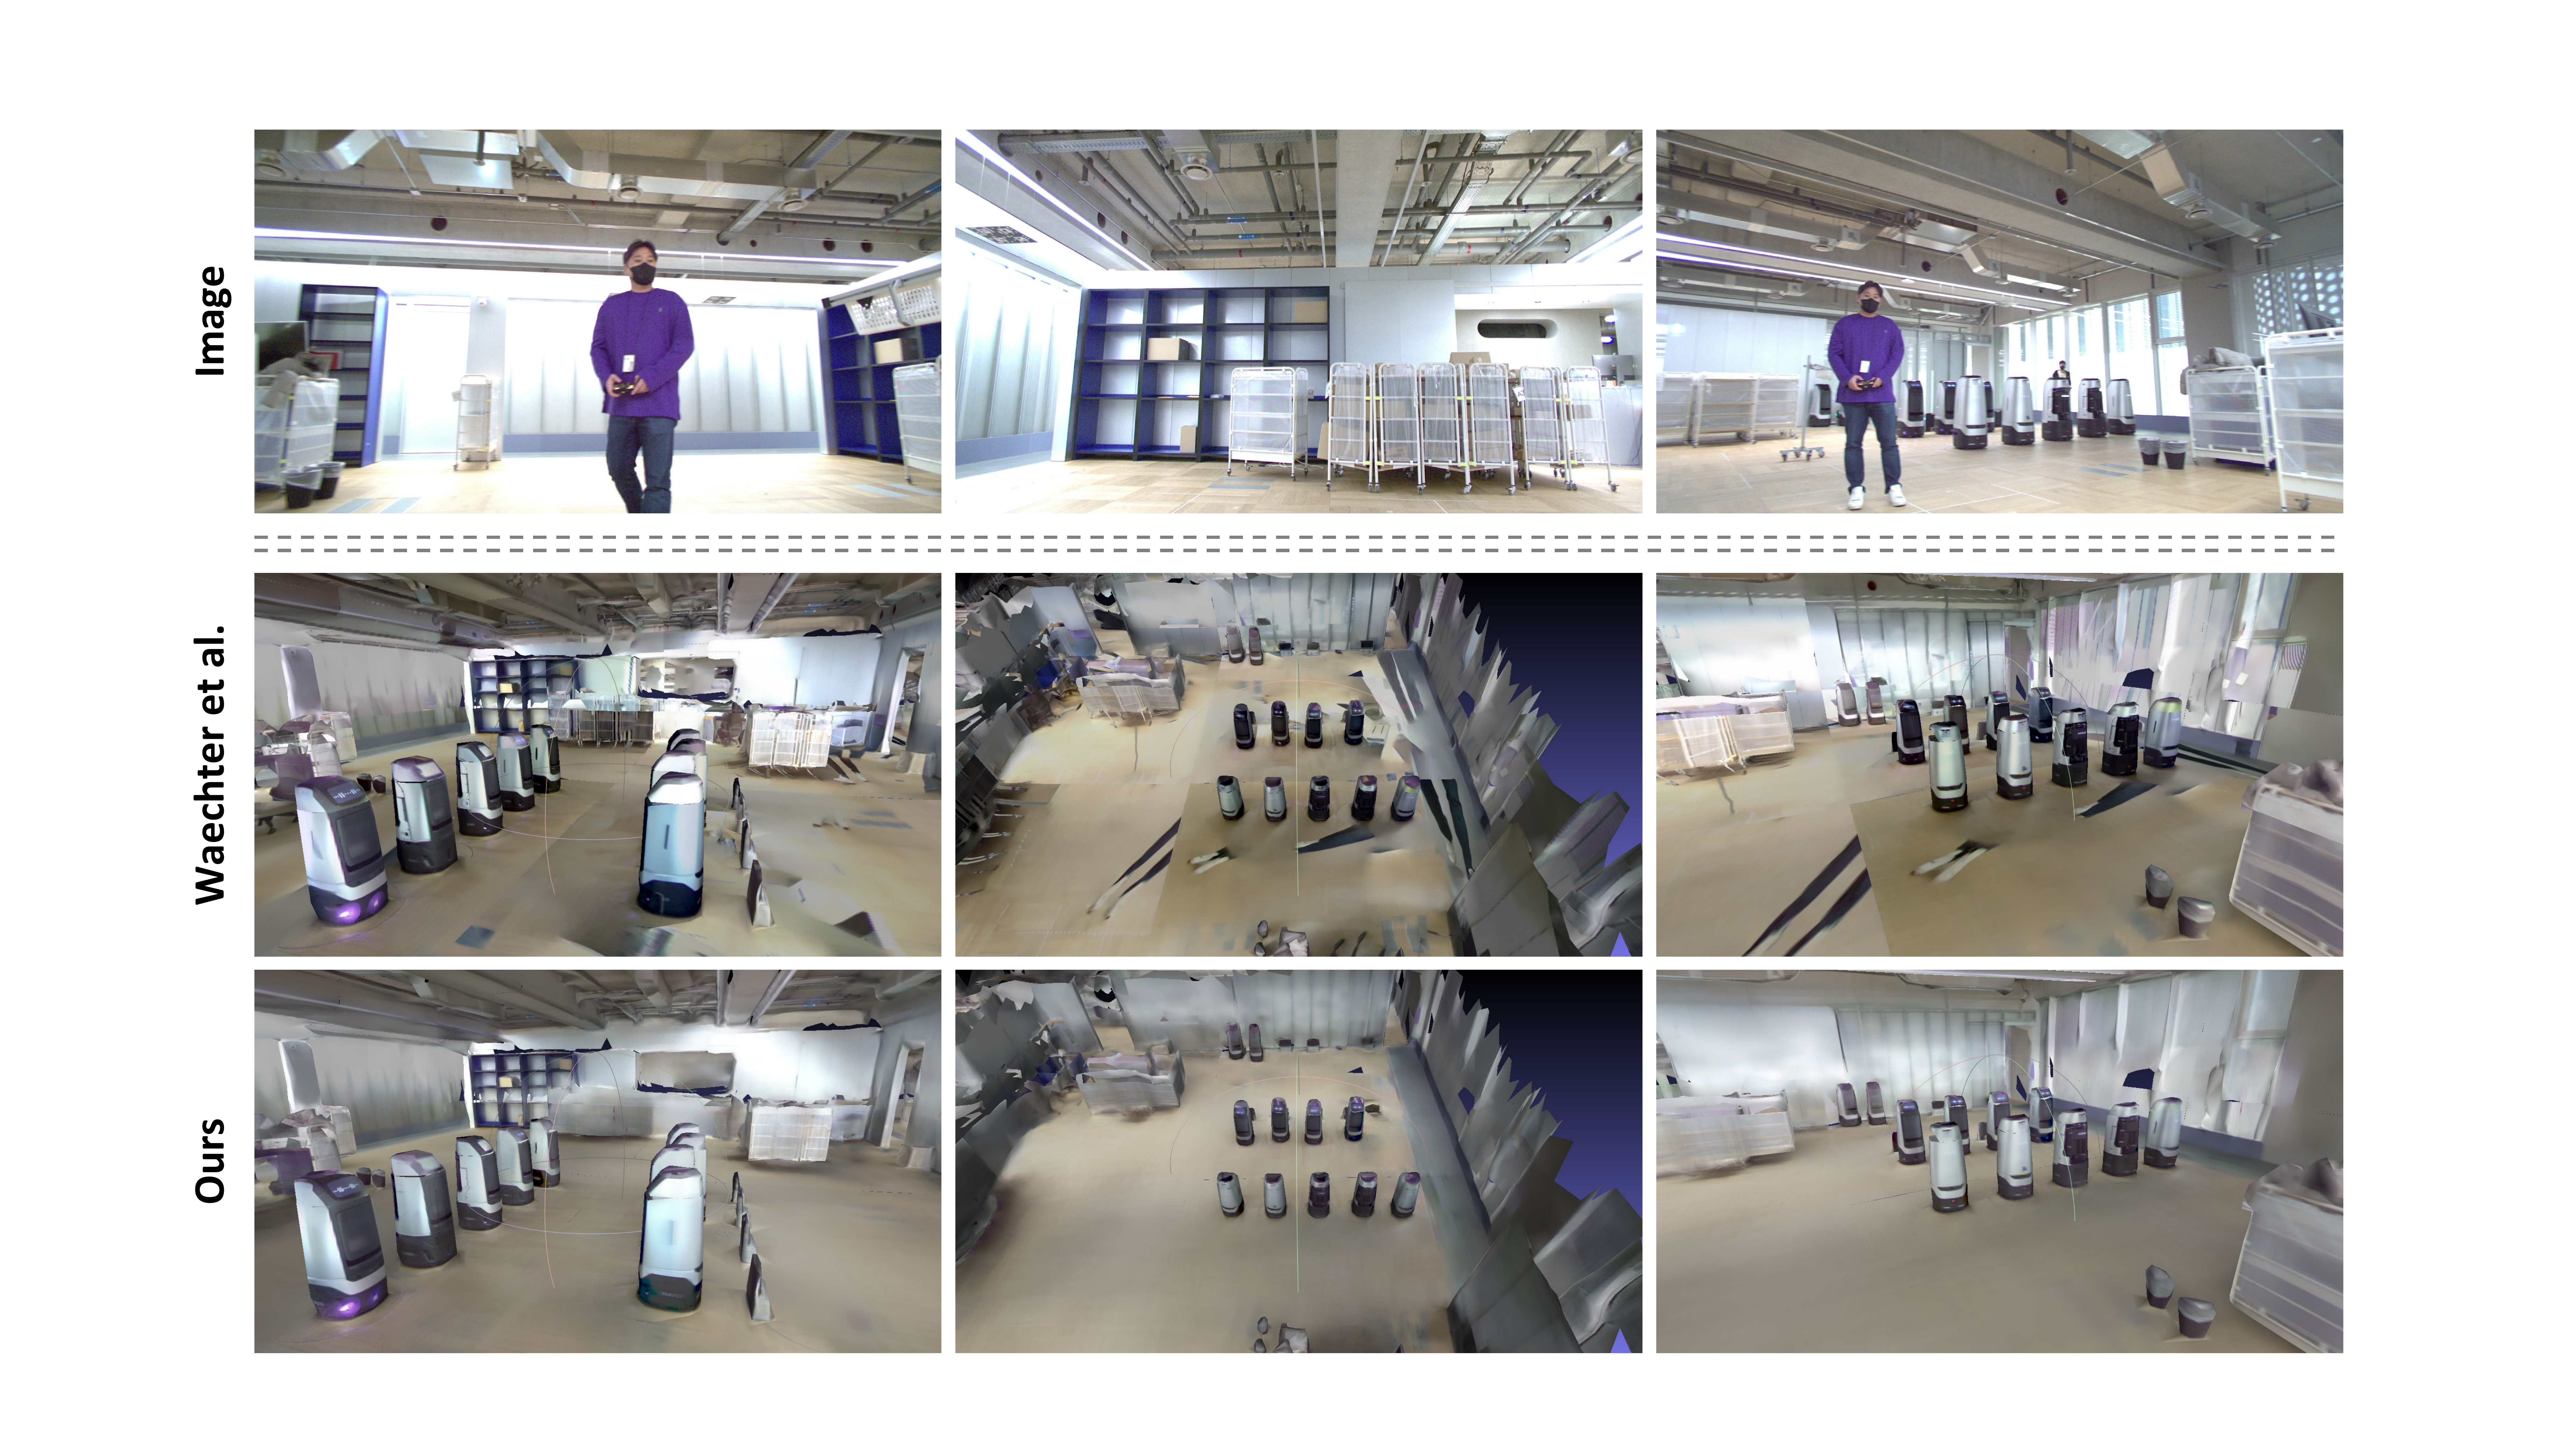}
    \vspace{-6mm}
   \caption{Example reconstruction results of 3D indoor scenes. Although our manuscript focuses on objects, we apply our method to reconstruct 3D indoor scenes from 2D images. We use 507 images for training. Our method can generate quite complete and smooth reconstruction results. In particular, we show the textured mesh reconstructed by classical texture reconstruction \cite{waechter2014TexRecon} (2nd row) and texture fine-tuning (3rd row) in Section 3.3. Our texture optimization method (3rd row) can remove ghosting effects and improve texture misalignment (2nd row) in indoor scenes.
   For future research, we will be able to extend our method to perform geometry reconstruction and texture optimization for 3D indoor scenes.  
   }
   % \vspace{-4mm}
   \label{fig:onecol}
\end{figure}

\newpage

\section{Qualitative Results}
 In Fig. \ref{fig:suppgeo2}, we show the reconstructed mesh for objects (\textit{robot arm 1}, \textit{robot arm2}, \textit{bike}, \textit{sofa}, \textit{camera stand}, \textit{plant}, and \textit{tree}) that are not included in the manuscript due to the limited space. Recently, MonoSDF \cite{yu2022monosdf} shows the state-of-the-art performance for the neural implicit surface reconstruction. We avoid using learning-based algorithms because they are expensive to acquire new training
datasets and time-consuming to train other neural networks. In contrast, MonoSDF exploits the power of pretrained Omnidata model \cite{eftekhar2021omnidata} which is trained by the large and diverse multi-task datasets. This pre-trained model can provide a surface normal and a depth map for a single image. While this pretrained model \cite{eftekhar2021omnidata} requires large amounts of data with expensive annotation costs and huge computational costs for training, MonoSDF succeeds to apply this model to boost its performance for surface reconstruction. However, we observe both the advantages and limitations of leveraging the pretrained model in our experiments. Figure \ref{fig:suppgeo1} visualizes the reconstructed mesh of MonoSDF including our method and VolSDF \cite{yariv2021volsdf}. Compared to ours and VolSDF, MonoSDF shows advances in reconstructing low-textured areas such as a back rest of the office chair and a paper box in the caffe stand. However, since its performance heavily relies on the quality of the pretrained model, it fails to reconstruct the accurate 3D geometry of plant and tree in Fig. \ref{fig:suppgeo2}.          
% bike: outdoor scene / sofa: large object 20 people can sit / tree: difficult scene, thin structure 
\newpage
\begin{figure}[h]
  \centering
    \includegraphics[width=\linewidth]{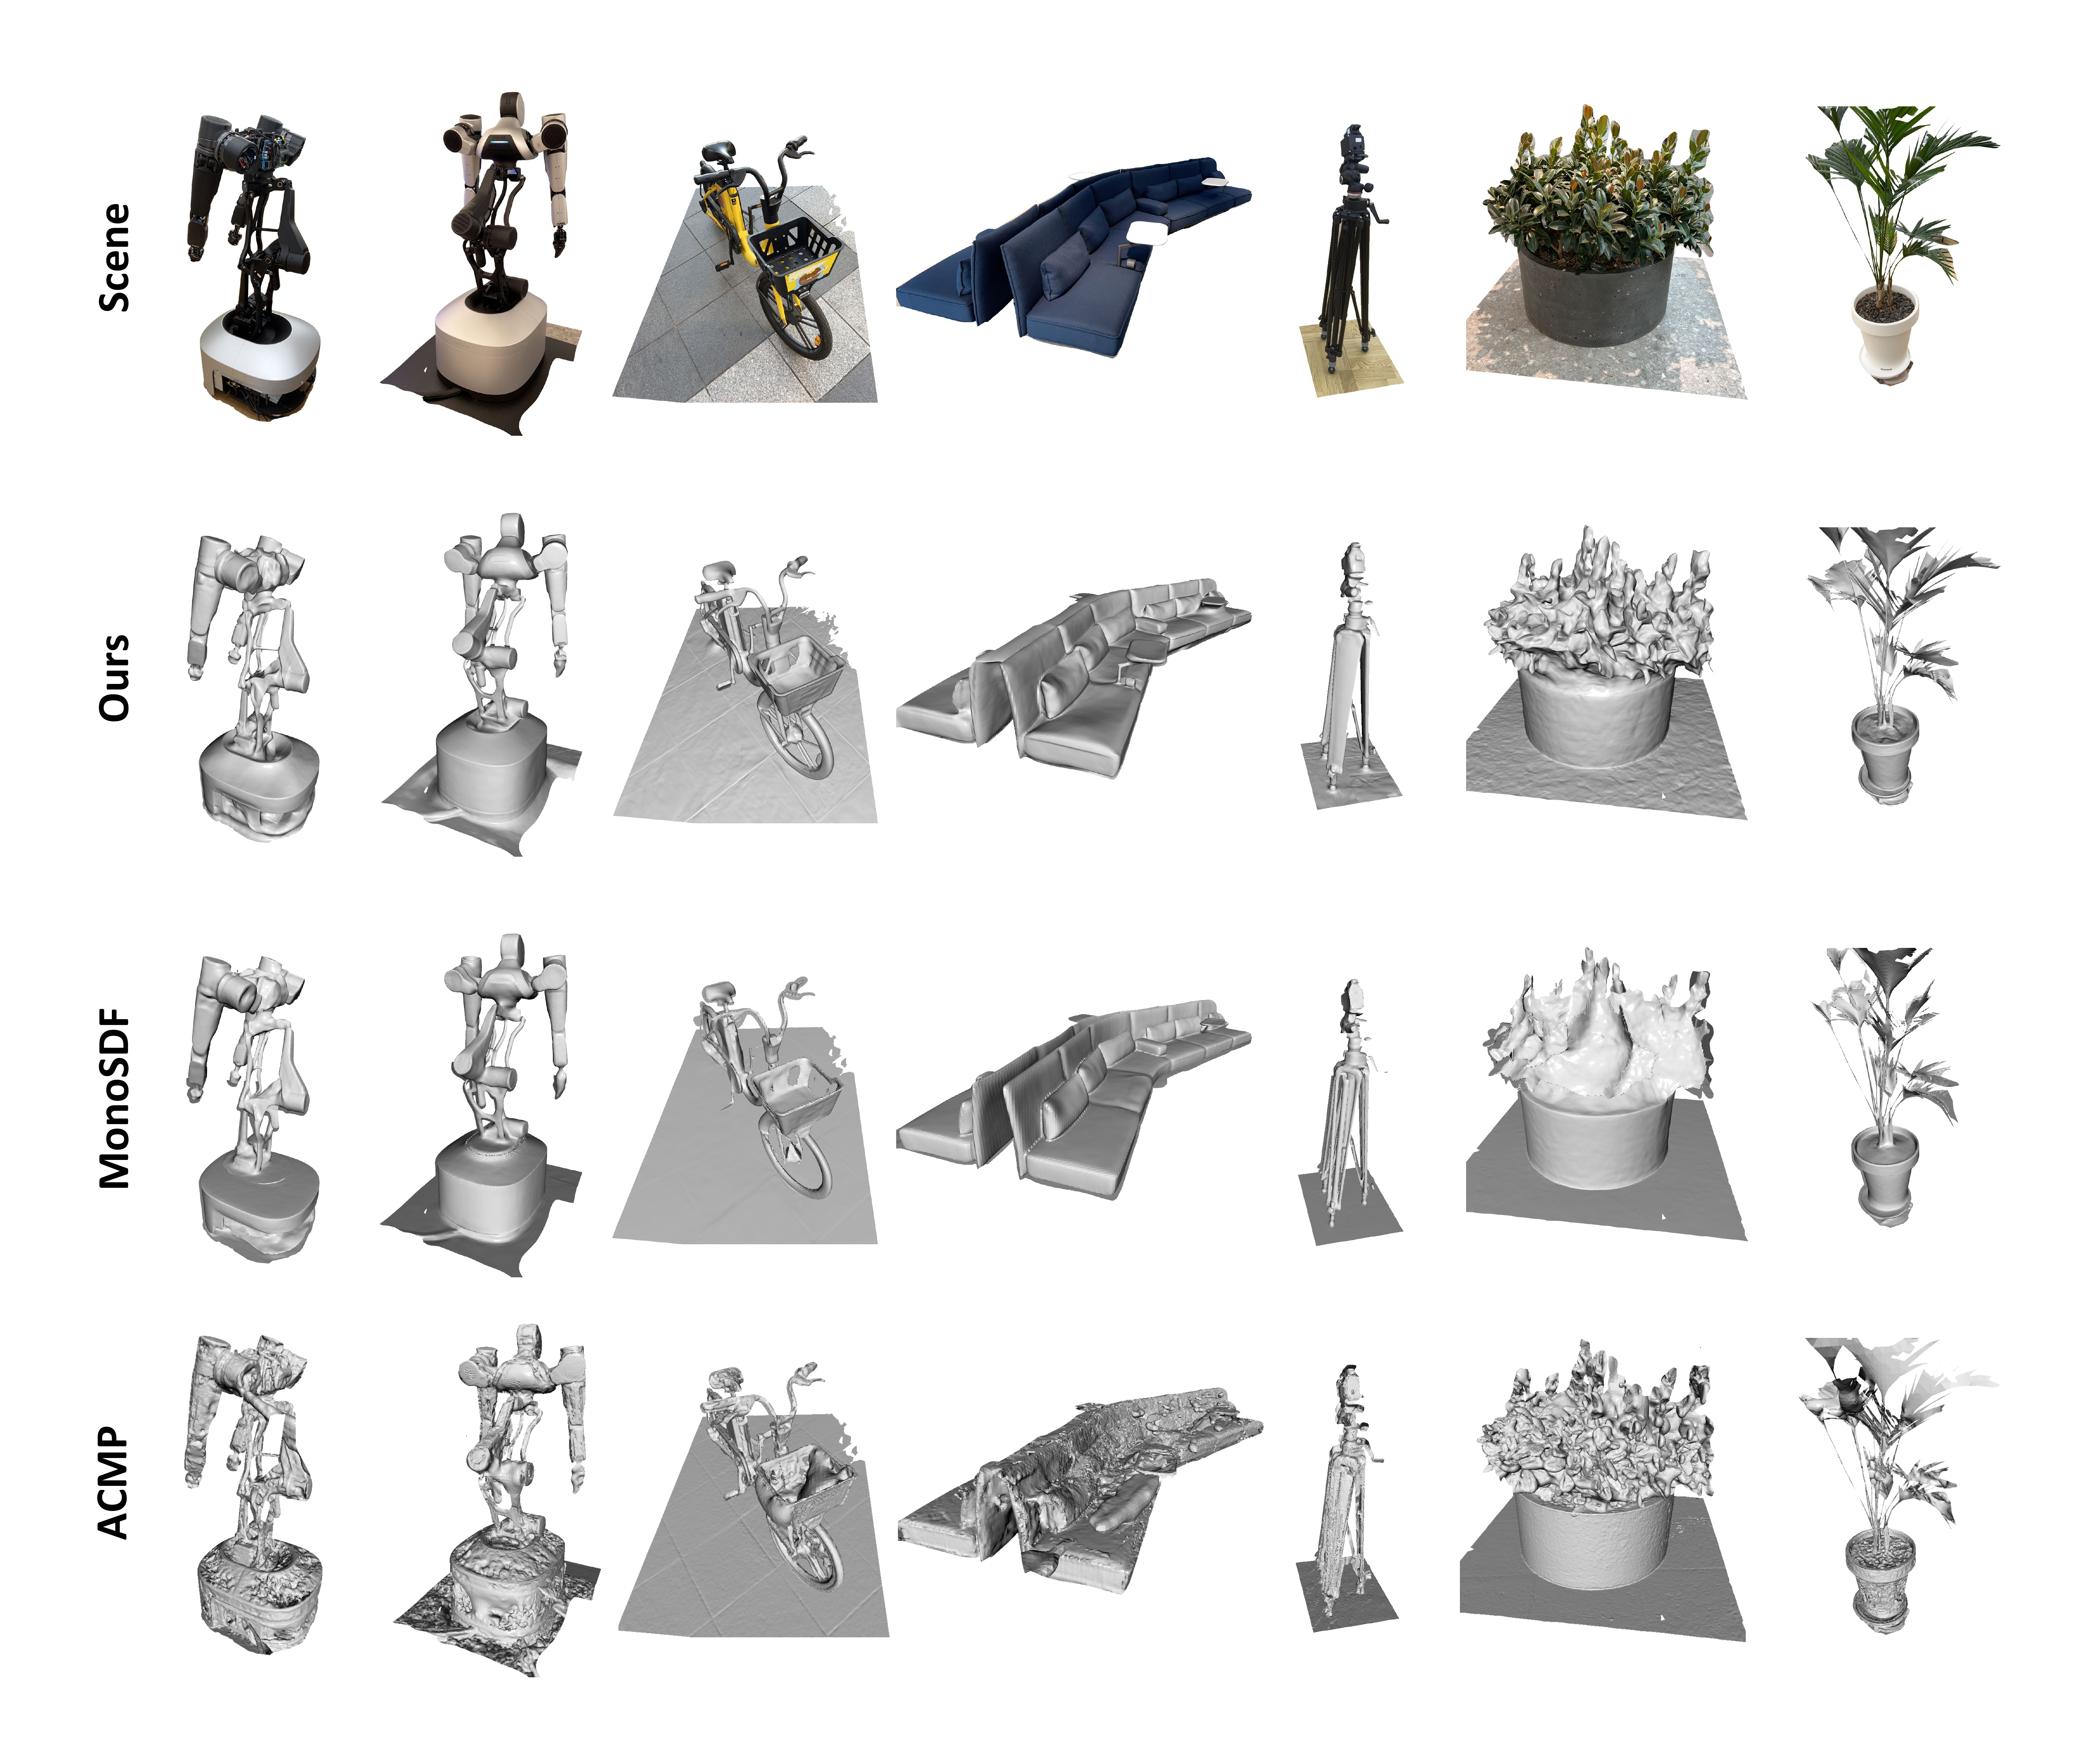}
    % \vspace{-3mm}
   \caption{From left to right, we show the reconstruction results of \textit{robot arm 1}, \textit{robot arm2}, \textit{bike}, \textit{sofa}, \textit{camera stand}, \textit{plant}, and \textit{tree}.  We notice that MonoSDF shows the high quality mesh for \textit{sofa} and \textit{camera stand} by improving the quality of low-textured regions. However, since the pretrained model provides bad quality of monocular depth and normal maps, Our method performs better than MonoSDF for \textit{plant}, \textit{tree}, and \textit{bike}}
   % \vspace{-4mm}
   \label{fig:suppgeo2}
\end{figure}

\newpage

\begin{figure}[h]
  \centering
    \includegraphics[width=0.7\linewidth]{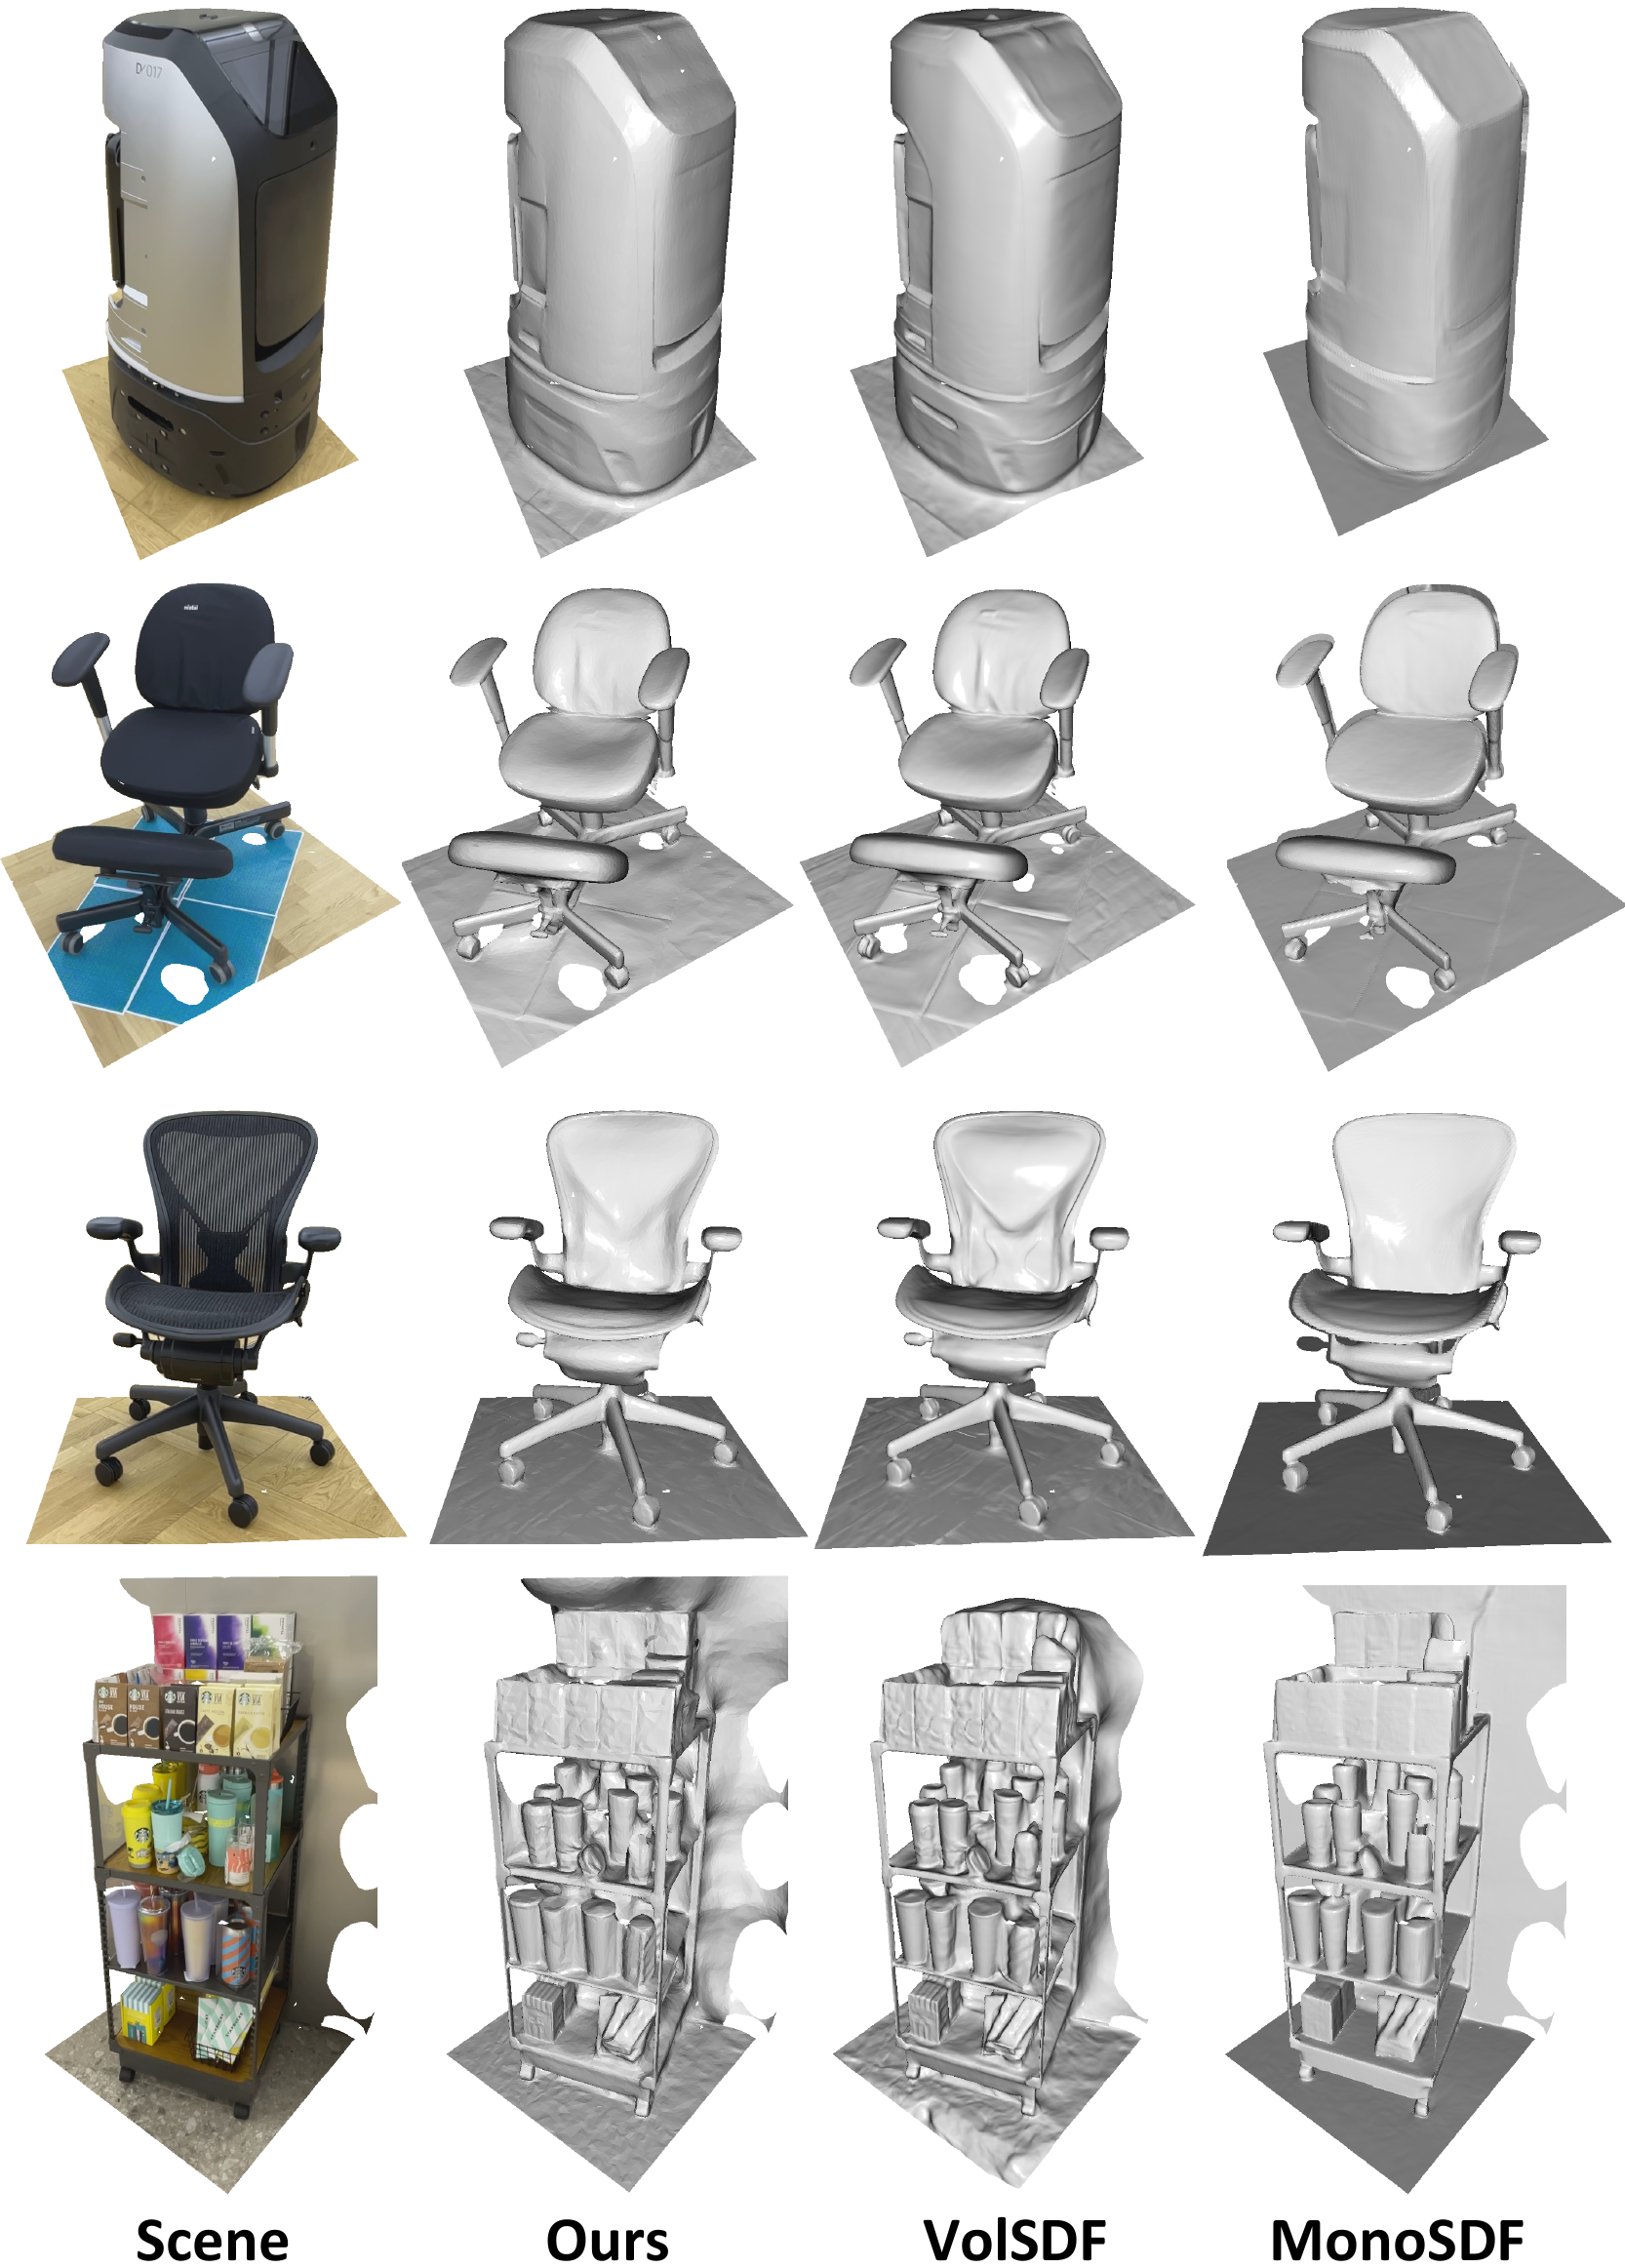}
    % \vspace{-3mm}
   \caption{Triangular mesh reconstructed by our method, VolSDF \cite{yariv2021volsdf}, and MonoSDF \cite{yu2022monosdf}.  From top to bottom, we show the results of \textit{delivery robot}, \textit{recliner chair}, \textit{office chair}, and \textit{cafe stand}. Here, MonoSDF can reconstruct the smooth space for low-textured regions compared to our method.}
   % \vspace{-4mm}
   \label{fig:suppgeo1}
\end{figure}

\newpage

\section{Run-time Analysis}
Our pipeline consists of three modules. First, \textbf{RGBD-aided SfM} (Sec.\:3.1) is imperative to refine initial poses due to noisy sensor data in Fig.\:5 (a). Without RGBD-aided SfM, our geometric reconstruction with initial poses shows poor quality in Fig.\:5 (b). 
% In the pipeline, our module is crucial. 
This process takes around 5 minutes on i9 CPU and Nvidia 2080 GPU to estimate accurate poses. In \textbf{Geometry Reconstruction} (Sec.\:3.2), both classical 3D reconstruction methods like MVS and depth Fusion (ACMP and TSDF-Fusion in Fig.\:6) fail to generate a decent mesh. Thus, we emphasize that applying neural geometry reconstruction after MVS is necessary to generate a high-quality mesh (our method in Fig.\:6). Overall, most of the time in our pipeline is spent on geometry reconstruction (around 10 hours on Nvidia V100 GPU).  
% However, if the MVS results are too noisy, it may have a negative effect on performance (e.g. scan37 in Table 2).
Then, the mesh simplification which only takes a few seconds. Lastly, in \textbf{Texture optimization} (Sec.\:3.3), 
%classical texture reconstruction [53] is more photorealistic and sharper than all different methods in Fig.7. 
the classical texture reconstruction \cite{waechter2014TexRecon} takes only a few seconds. Fig.\:7 and Table\:1. show that our proposed texture fine-tuning solves the seams and texture misalignment issues often seen with this classical method. Our proposed module, which takes less than 15 minutes on i9 CPU and Nvidia 2080 GPU, can generate visually realistic textures. 

%%%%%%%%% REFERENCES
{\small
\bibliographystyle{ieee_fullname}
\bibliography{main}
}

\end{document}
